# Supplementary material for: Controlling Latent Diffusion Using Latent CLIP
Source: arXiv:2503.08455 source file (2025-03-11)
Supplement: Supplementary file 1 [file appendix_exp2_t2i.tex]

\begin{table}[h!]
\centering
\caption{Extended quantitative results on T2I-CompBench.} 
\label{tab:appendix_t2icompbenchfull}
\resizebox{\columnwidth}{!}{ 
\begin{tabular}
{lccccccc} % Added an extra column here
\toprule
\multicolumn{1}{c}
{\multirow{2}{*}{\textbf{ Reward Model}}} & \multicolumn{3}{c}{\textbf{ Attribute Binding }} & \multicolumn{2}{c}{\textbf{ Object Relationship}} & \multirow{2}{*}{\textbf{ Complex$\uparrow$}} & \multirow{2}{*}{\textbf{ Aesthetic$\uparrow$}} \\ % Added Aesthetic column here
\cmidrule(lr){2-4}\cmidrule(lr){5-6}

&
{\textbf{ Color $\uparrow$ }} &
{\textbf{ Shape$\uparrow$}} &
{\textbf{ Texture$\uparrow$} }&
{\textbf{ Spatial$\uparrow$} }&
{\textbf{ Non-Spatial$\uparrow$}} &
\\
\midrule
Base (SDXL-Turbo)  & 0.6160 & 0.4370 & 0.6010 & 0.2440 & 0.3118 & 0.4244 & 5.5053 \\ % Add values or placeholders (e.g., "--") for Aesthetic
ReNO & 0.7840 & 0.5929 & 0.7427 & 0.2496 & 0.3157 & 0.4674 & 5.6991 \\

\midrule
{\textbf{CLIPScore}} \\
\midrule

\rowcolor{lavender}
{Latent-ViT-B-8-512}  & 0.6823 & 0.5372 & 0.6867 & 0.2500 & 0.3176 & 0.4447 & 5.5422 \\
\rowcolor{lavender}
{Latent-ViT-B-4-512-plus} & 0.6887 & 0.5428 & 0.6996 & 0.2435 & 0.3173 & 0.4450 & 5.5460 \\
%\midrule
CLIP-ViT-B-32-laion2B-s34B-b79K & 0.6917 & 0.5407 & 0.6792 & 0.2338 & 0.3202 & 0.4413 & 5.5607 \\
CLIP-ViT-B-16-plus-240-laion400m-e32    & 0.6829 & 0.5491 & 0.6936 & 0.2408 & 0.3195 & 0.4343 & 5.5399 \\
CLIP-ViT-B-16-laion2B-s34B-b88K & 0.6802 & 0.5387 & 0.6894 & 0.2314 & 0.3173 & 0.4300 & 5.5566 \\
CLIP-ViT-B-32-256x256-DataComp-s34B-b86K & 0.6736 & 0.5330 & 0.6847 & 0.2403 & 0.3166 & 0.4284 & 5.5567 \\
CLIP-ViT-B-16-DataComp.XL-s13B-b90K & 0.6741 & 0.5340 & 0.6844 & 0.2395 & 0.3160 & 0.4466 & 5.5527 \\
CLIP-ViT-L-14-laion2B-s32B-b82K & 0.6964 & 0.5309 & 0.6815 & 0.2529 & 0.3151 & 0.4364 & 5.5689 \\
CLIP-ViT-H-14-laion2B-s32B-b79K & 0.6985 & 0.5443 & 0.6856 & 0.2585 & 0.3160 & 0.4358 & 5.5481 \\
CLIP-ViT-g-14-laion2B-s34B-b88K  & 0.6888 & 0.5355 & 0.6871 & 0.2337 & 0.3158 & 0.4419 & 5.5562 \\

\midrule
{\textbf{PickScore}} \\
\midrule

\rowcolor{lavender}
{Latent-ViT-B-8-512}  & 0.6532 & 0.5070 & 0.6459 & 0.2541 & 0.3142 & 0.4456 & 5.5983 \\
\rowcolor{lavender}
{Latent-ViT-B-4-512-plus}  & 0.6825 & 0.5177 & 0.6538 & 0.2539 & 0.3143 & 0.4351 & 5.6670 \\
%\midrule
CLIP-ViT-B-32-laion2B-s34B-b79K & 0.6534 & 0.5079 & 0.6469 & 0.2354 & 0.3122 & 0.4223 & 5.6618 \\
CLIP-ViT-B-16-plus-240-laion400m-e32  & 0.6980 & 0.5604 & 0.7029 & 0.2363 & 0.3192 & 0.4485 & 5.6046 \\
CLIP-ViT-B-16-laion2B-s34B-b88K & 0.6673 & 0.5061 & 0.6557 & 0.2394 & 0.3132 & 0.4371 & 5.6797 \\

CLIP-ViT-B-32-256x256-DataComp-s34B-b86K & 0.6645 & 0.5122 & 0.6574 & 0.2384 & 0.3131 & 0.4192 & 5.6641 \\
CLIP-ViT-B-16-DataComp.XL-s13B-b90K & 0.6508 & 0.5001 & 0.6546 & 0.2601 & 0.3124 & 0.4313 & 5.6710 \\
CLIP-ViT-L-14-laion2B-s32B-b82K  & 0.6563 & 0.5010 & 0.6535 & 0.2470 & 0.3131 & 0.4191 & 5.6363 \\
CLIP-ViT-H-14-laion2B-s32B-b79K   & 0.6588 & 0.5193 & 0.6593 & 0.2436 & 0.3116 & 0.4291 & 5.6962 \\
\bottomrule
\end{tabular}
}
%\vspace{-1em}
\end{table}
