# Supplementary material for: Controlling Latent Diffusion Using Latent CLIP
Source: arXiv:2503.08455 source file (2025-03-11)
Supplement: Supplementary file 2 [file appendix_interpolate.tex]

\begin{table}[htbp]
  \caption{Extended classification performance of LatentCLIP and traditional CLIP models across different workflows and interpolation methods. (1) refers to latents directly using interpolated representations, while (2) involves resizing generated images and decoding them back into latent space.}
  \label{tab:appendix_interpolation_comparison_table}
  \centering
  \resizebox{\textwidth}{!}{%
  \begin{tabular}{llcccc}
    \toprule
    \textbf{Model} & \textbf{Interpolation} & \multicolumn{2}{c}{\textbf{Basic Workflow}} & \multicolumn{2}{c}{\textbf{Advanced Workflow}} \\
    \cmidrule(lr){3-4} \cmidrule(lr){5-6}
    & & \textbf{Top-1} & \textbf{Top-5} & \textbf{Top-1} & \textbf{Top-5} \\
    \midrule
    \multirow{5}{*}{(1) Latent-ViT-B-8-512} 
        & area & 21.04 & 38.46 & 25.47 & 46.17 \\
        & bilinear & 50.34 & 75.60 & 44.74 & 70.24 \\
        & bicubic & 49.55 & 74.94 & 35.99 & 60.63 \\
        & nearest-exact & 55.54 & 80.25 & 38.94 & 64.39 \\
        & nearest & 55.93 & 80.54 & 38.85 & 64.35 \\
    \cmidrule(lr){2-6} % Adds a line from the second to the last column
    
    %\midrule
    \multirow{5}{*}{(1) Latent-ViT-B-4-512-plus}
        & area & 15.00 & 28.74 & 17.89 & 34.31 \\
        & bilinear & 43.58 & 68.45 & 44.86 & 70.37 \\
        & bicubic & 50.26 & 75.90 & 41.97 & 67.14 \\
        & nearest-exact & 62.67 & 85.66 & 49.12 & 75.02 \\
        & nearest & 62.86 & 85.78 & 49.20 & 75.08 \\
        
    \midrule
    \midrule 
    
    \multirow{1}{*}{CLIP-ViT-B-32-laion2B-s34B-b79K} 
       & - & 79.81 & 95.16 & 73.53 & 92.91 \\
        
    \multirow{1}{*}{CLIP-ViT-B-16-plus-240-laion400m-e32} 
        & - & 80.91 & 95.84 & 75.42 & 94.04 \\
        
    \multirow{1}{*}{CLIP-ViT-B-16-laion2B-s34B-b88K} 
        & - & 81.53 & 95.87 & 76.19 & 94.14 \\
        
    \multirow{1}{*}{CLIP-ViT-B-32-256x256-DataComp-s34B-b86K} 
        & - & 82.16 & 95.95 & 76.89 & 94.24 \\
        
    \multirow{1}{*}{CLIP-ViT-B-16-DataComp.XL-s13B-b90K} 
       & - & 83.10 & 96.46 & 78.18 & 94.75 \\
        
    % Regular midrule for separation between the two sections
    \multirow{1}{*}{CLIP-ViT-L-14-laion2B-s32B-b82K} 
        & - & 83.91 & 96.70 & 79.83 & 95.52 \\
    %\cmidrule(lr){2-6} % Line from the second to the last column for the last two models
    
    \multirow{1}{*}{CLIP-ViT-H-14-laion2B-s32B-b79K} 
        & - & 85.24 & 97.10 & 81.47 & 96.02 \\
        
    \multirow{1}{*}{CLIP-ViT-g-14-laion2B-s34B-b88K} 
        & - & 84.66 & 96.89 & 81.38 & 95.98 \\
        
    \midrule
    \midrule  % Regular midrule for separation between the two sections
    
    \multirow{1}{*}{(2) Latent-ViT-B-8-512} 
        & - & 79.93 & 95.55  & 74.12 & 93.17 \\
    %\cmidrule(lr){2-6} % Line from the second to the last column for the last two models
    \multirow{1}{*}{(2) Latent-ViT-B-4-512-plus} 
        & - & 82.58 & 96.40  & 78.28 & 94.83 \\
        
    \bottomrule
  \end{tabular}
  }
\end{table}

\iffalse
    CLIP-ViT-B-32-laion2B-s34B-b79K & 0.67 & 0.90 \\
    CLIP-ViT-B-16-plus-240-laion400m-e32 & 0.69 & 0.91 \\
    CLIP-ViT-B-16-laion2B-s34B-b88K & 0.70 & 0.92 \\
    CLIP-ViT-B-32-256x256-DataComp-s34B-b86K & 0.73 & 0.93 \\
    CLIP-ViT-B-16-DataComp.XL-s13B-b90K & 0.73 & 0.93 \\
    CLIP-ViT-L-14-laion2B-s32B-b82K & 0.75 & 0.94 \\
    CLIP-ViT-H-14-laion2B-s32B-b79K & 0.78 & 0.95 \\
    CLIP-ViT-g-14-laion2B-s34B-b88K & 0.78 & 0.95 \\
\fi
