# Supplementary material for: Controlling Latent Diffusion Using Latent CLIP
Source: arXiv:2503.08455 source file (2025-03-11)
Supplement: Supplementary file 3 [file appendix_exp2_geneval.tex]

\begin{table}[h!]
\centering
\caption{Extended quantitative results on GenEval.} 
\label{tab:appendix_geneval}
\resizebox{\columnwidth}{!}{ 
\begin{tabular}
{lcccccccc} % Added an extra column here
\toprule

\textbf{Model} &
{\textbf{ Mean $\uparrow$ }} &
{\textbf{ Single$\uparrow$}} &
{\textbf{ Two$\uparrow$}} &
{\textbf{ Counting$\uparrow$}} &
{\textbf{ Colors$\uparrow$}} &
{\textbf{ Position$\uparrow$}} &
{\textbf{ Color Attribution$\uparrow$}} &
{\textbf{ Aesthetic$\uparrow$}}\\
\\
\midrule
Base (SDXL-Turbo) & 0.5390 & 0.9938 & 0.6566 & 0.4531 & 0.8457 & 0.0850 & 0.2000 & 5.3918 \\ % Add values or placeholders (e.g., "--") for Aesthetic
ReNO & 0.6408 & 0.9906 & 0.8586 & 0.6219 & 0.8989 & 0.1150 & 0.3600 & 5.5750 \\

\midrule
{\textbf{CLIPScore}} \\
\midrule

\rowcolor{lavender}
{Latent-ViT-B-8-512} & 0.6023 & 0.9844 & 0.7778 & 0.5312 & 0.8856 & 0.1200 & 0.3150 & 5.4000 \\
\rowcolor{lavender}
{Latent-ViT-B-4-512-plus}  & 0.6233 & 0.9906 & 0.8207 & 0.5969 & 0.8989 & 0.1350 & 0.2975 & 5.4000 \\
%\midrule
CLIP-ViT-B-32-laion2B-s34B-b79K & 0.6109 & 0.9875 & 0.8207 & 0.5938 & 0.8883 & 0.1100 & 0.2650 & 5.4343 \\
CLIP-ViT-B-16-plus-240-laion400m-e32 & 0.6208 & 0.9938 & 0.8056 & 0.5531 & 0.9149 & 0.1350 & 0.3225 & 5.4169 \\
CLIP-ViT-B-16-laion2B-s34B-b88K & 0.5937 & 0.9969 & 0.7854 & 0.5531 & 0.8670 & 0.1125 & 0.2475 & 5.4353 \\
CLIP-ViT-B-32-256x256-DataComp-s34B-b86K & 0.5898 & 0.9906 & 0.7828 & 0.5500 & 0.8777 & 0.1100 & 0.2275 & 5.4342 \\
CLIP-ViT-B-16-DataComp.XL-s13B-b90K & 0.6053 & 0.9875 & 0.8081 & 0.5844 & 0.9096 & 0.1100 & 0.2325 & 5.4372 \\
CLIP-ViT-L-14-laion2B-s32B-b82K & 0.6281 & 0.9938 & 0.8384 & 0.6188 & 0.8830 & 0.1350 & 0.3000 & 5.4436 \\
CLIP-ViT-H-14-laion2B-s32B-b79K & 0.6252 & 0.9844 & 0.8283 & 0.6188 & 0.9149 & 0.1025 & 0.3025 & 5.4314 \\
CLIP-ViT-g-14-laion2B-s34B-b88K  & 0.6190 & 1.0000 & 0.8207 & 0.6031 & 0.9176 & 0.1075 & 0.2650 & 5.4438 \\

\midrule
{\textbf{PickScore}} \\
\midrule

\rowcolor{lavender}
{Latent-ViT-B-8-512} & 0.6050 & 1.0000 & 0.7677 & 0.5750 & 0.9122 & 0.1000 & 0.2750 & 5.3980 \\
\rowcolor{lavender}
{Latent-ViT-B-4-512-plus} & 0.6169 & 0.9938 & 0.7879 & 0.6312 & 0.8963 & 0.1325 & 0.2600 & 5.4982 \\
%\midrule
CLIP-ViT-B-32-laion2B-s34B-b79K & 0.6032 & 0.9938 & 0.7803 & 0.5562 & 0.9016 & 0.0975 & 0.2900 & 5.4910 \\
CLIP-ViT-B-16-plus-240-laion400m-e32 & 0.6191 & 1.0000 & 0.8283 & 0.5813 & 0.9149 & 0.1100 & 0.2800 & 5.4755 \\
CLIP-ViT-B-16-laion2B-s34B-b88K & 0.6033 & 0.9938 & 0.7879 & 0.5750 & 0.8883 & 0.1000 & 0.2750 & 5.5058 \\
CLIP-ViT-B-32-256x256-DataComp-s34B-b86K & 0.6009 & 0.9938 & 0.8030 & 0.5781 & 0.8856 & 0.1050 & 0.2400 & 5.4951 \\
CLIP-ViT-B-16-DataComp.XL-s13B-b90K & 0.5961 & 1.0000 & 0.7500 & 0.5781 & 0.8883 & 0.1000 & 0.2600 & 5.5172 \\
CLIP-ViT-L-14-laion2B-s32B-b82K  & 0.6141 & 1.0000 & 0.7980 & 0.6062 & 0.8856 & 0.1425 & 0.2525 & 5.5026 \\
CLIP-ViT-H-14-laion2B-s32B-b79K & 0.6184 & 1.0000 & 0.8283 & 0.6188 & 0.8910 & 0.1100 & 0.2625 & 5.5299 \\

\bottomrule
\end{tabular}
}
%\vspace{-1em}
\end{table}
